# Supplementary material for: Rate constants from instanton theory via a microcanonical approach
Source: arXiv:2009.03547 source file (2020-09-08)
Supplement: Supplementary file 1 [file supp.pdf]

# Supporting information to:
# Rate constants from instanton theory via a microcanonic approach

Sean R. McConnell,[1] Andreas Löhle,[1] and Johannes Kästner[1]
*Institute for Theoretical Chemistry, University of Stuttgart, Pfaffenwaldring 55, 70569 Stuttgart,Germany, kaestner@theochem.uni-stuttgart.de*

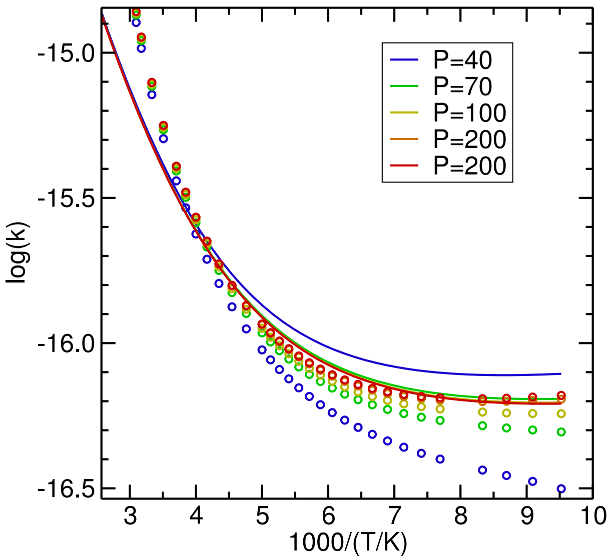


FIG. 1. Dependence of the rate constants on the number of images $P$ of the instanton for the method of directly solving the stability matrix differential equation. Dots are the rate constants obtained with direct canonic instanton theory at the respective number of images.

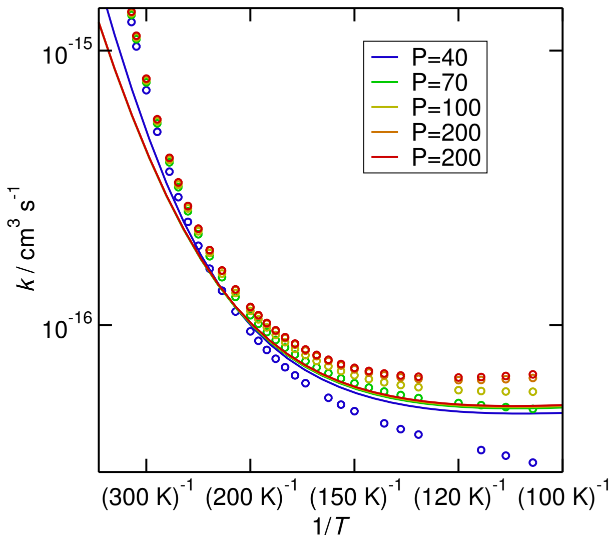


FIG. 2. Dependence of the rate constants on the number of images $P$ of the instanton for eigenvalue tracing. Dots are the rate constants obtained with direct canonic instanton theory at the respective number of images.

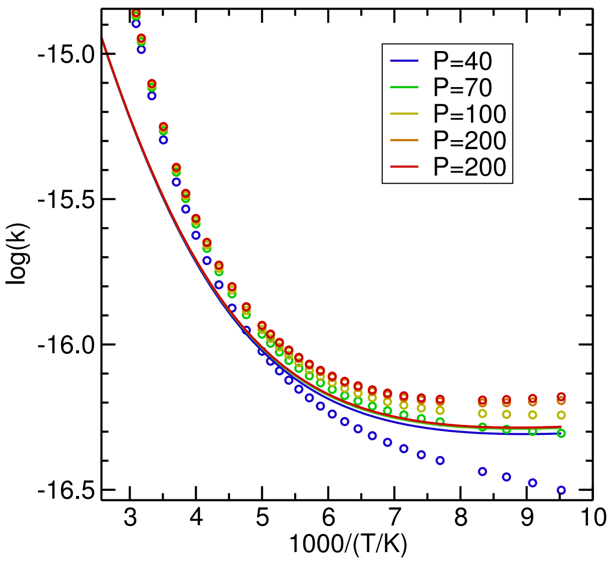


FIG. 3. Dependence of the rate constants on the number of images $P$ of the instanton for frequency averaging. Dots are the rate constants obtained with direct canonic instanton theory at the respective number of images.

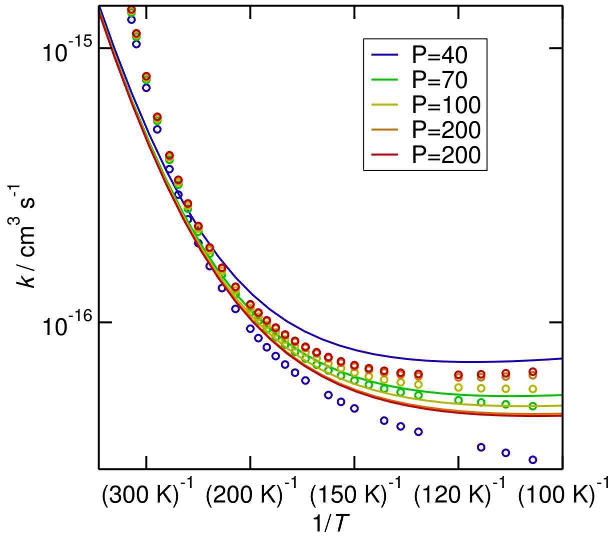


FIG. 4. Dependence of the rate constants on the number of images $P$ of the instanton for obtaining $\sigma$ from the method product of eigenvalues of the full Hessian. Dots are the rate constants obtained with direct canonic instanton theory at the respective number of images.
